# Supplementary material for: DCA-Bench: A Benchmark for Dataset Curation Agents
Source: arXiv:2406.07275 source file (2025-05-26)
Supplement: Supplementary file 1 [file relatedworks.tex]

{\subsection{More Discussion on Dataset Quality Management Related Works}
\label{more-related-works}
\up{
The FAIR principle \citep{wilkinsonFAIRGuidingPrinciples2016} is an influential framework focused on enhancing Findability (Metadata and data should be easy to find for both humans and computers), Accessibility (Information about how they can be accessed, possibly including authentication and authorization), Interoperability (metadata need to follow the same format to be interoperable), and Reusability (metadata and data should be well-described) of digital assets. \textbf{While the FAIR principle can make datasets more usable through proper credit and citation mechanisms, it is somewhat too general regarding other dataset issues we have discovered in datasets found in the wild.} FAIR mentions in R1 that “data are richly described with a plurality of accurate and relevant attributes” and in R1.3 that “(Meta)data meet domain-relevant community standards.” \textbf{However, these statements are quite general and lack the detail needed to address the specific issues found in real-world datasets and to provide detailed guidance for dataset creators.} Therefore, instead of a top-down approach, we believe that collecting and analyzing datasets in the wild as examples can provide a more detailed and practical understanding of common issues faced by dataset users, as we discussed in~\ref{define-data-quality}. 

Other relevant works on general dataset management include~\citet{holland2020dataset}, which simplifies data analysis and improves AI model quality by providing a comprehensive overview of dataset characteristics, and~\citet{hutchinson2021accountability}, which enhances accountability in AI systems by making the often overlooked processes behind dataset creation visible. However, these topics are largely covered by~\citet{gebru2021datasheets}.

}
